# Supplementary material for: Conformational Nonequilibrium Enzyme Kinetics: Generalized Michaelis-Menten Equation
Source: arXiv:1703.02011 ancillary file (2017-05-16)
Supplement: Supplementary file 1 [file supporting-info.pdf]

# Supporting information for: Conformational Nonequilibrium Enzyme Kinetics: Generalized Michaelis–Menten Equation

D. Evan Piephoff,[†,‡] Jianlan Wu,[†,‡] and Jianshu Cao[*,†]

†*Department of Chemistry, Massachusetts Institute of Technology, Cambridge, Massachusetts 02139, United States*

‡*Contributed equally to this work*

E-mail: jianshu@mit.edu

## Four-Site Model Calculations

Here, we provide detailed calculations for a $2 \times 2$, four-site model for enzyme turnover. We reported an equivalent solution for this model in ref 15 of the main text, but below, we give explicit results for the substrate concentration dependence of the turnover rate. Using the decomposed representation of the scheme, the MFPT can be written as

$$\langle t \rangle = \sum_{i=1}^{N} \left[ \tau_{\mathrm{E}_i}^{\mathrm{eff}} + \tau_{\mathrm{ES}_i}^{\mathrm{eff}} \right] F_{i,0} \tag{S.1}$$

For the $2\times 2$ network, $k_{i,2}^{\text{eff}} = k_{i,2}$ and $K_{i,\text{M}}^{\text{eff}} = [k_{i,-1}+k_{i,2}+\gamma_{(-1)^{i+1},2}(1-k_{i,1}^0/k_{-i+3,1}^0)]/(k_{i,1}^0[\text{S}])$. Thus,

$$\begin{aligned}\langle t\rangle = &\left[\frac{k_{1,-1}+k_{1,2}+\gamma_{1,2}(1-k_{1,1}^0/k_{2,1}^0)}{k_{1,1}^0 k_{1,2}[\text{S}]}+\frac{1}{k_{1,2}}\right]F_{1,0}\\ &+\left[\frac{k_{2,-1}+k_{2,2}+\gamma_{-1,2}(1-k_{2,1}^0/k_{1,1}^0)}{k_{2,1}^0 k_{2,2}[\text{S}]}+\frac{1}{k_{2,2}}\right]F_{2,0}\end{aligned} \tag{S.2}$$

where the initial fluxes are given by

$$F_{1,0} = f_{1,0}+\frac{f_{1,1}}{[\text{S}]+s_1} \tag{S.3}$$

$$F_{2,0} = 1-F_{1,0} \tag{S.4}$$

with

$$f_{1,0} = \frac{k_{1,2}\gamma_{-1,2}}{k_{1,2}\gamma_{-1,2}+k_{2,2}\gamma_{1,2}} \tag{S.5}$$

$$f_{1,1} = -\frac{k_{1,2}k_{2,2}\gamma_{1,2}\gamma_{-1,2}}{(k_{1,2}\gamma_{-1,2}+k_{2,2}\gamma_{1,2})^2}\left(\frac{\gamma_{1,1}}{\gamma_{1,2}}K_{1,\text{M}}-\frac{\gamma_{-1,1}}{\gamma_{-1,2}}K_{2,\text{M}}\right) \tag{S.6}$$

$$s_1 = \frac{\gamma_{1,1}}{k_{1,1}^0}+\frac{\gamma_{-1,1}}{k_{2,1}^0}+\frac{k_{2,2}\gamma_{1,1}K_{1,\text{M}}+k_{1,2}\gamma_{-1,1}K_{2,\text{M}}}{k_{1,2}\gamma_{-1,2}+k_{2,2}\gamma_{1,2}} \tag{S.7}$$

where $K_{i,\text{M}} = (k_{i,-1}+k_{i,2})/k_{i,1}^0$. The turnover rate is then expressed as

$$v = \left[A_0+\frac{B_0}{[\text{S}]}+\frac{B_1}{[\text{S}]+s_1}\right]^{-1} \tag{S.8}$$

where the reduced parameters are given by

$$A_0 = \frac{\gamma_{1,2}+\gamma_{-1,2}}{k_{1,2}\gamma_{-1,2}+k_{2,2}\gamma_{1,2}} \tag{S.9}$$

$$B_0 = \frac{(\gamma_{1,1}+\gamma_{-1,1})K_{1,\text{M}}K_{2,\text{M}}[1+\gamma_{1,2}/(k_{1,1}^0K_{1,\text{M}})+\gamma_{-1,2}/(k_{2,1}^0K_{2,\text{M}})]}{\gamma_{1,1}k_{2,2}\mathcal{K}_1+\gamma_{-1,1}k_{1,2}\mathcal{K}_2} \tag{S.10}$$

$$B_1 = \frac{(k_{1,2}k_{2,2})^2\gamma_{1,2}\gamma_{-1,2}(\gamma_{1,1}K_{1,\text{M}}/\gamma_{1,2}-\gamma_{-1,1}K_{2,\text{M}}/\gamma_{-1,2})(\mathcal{K}_1\Gamma_1/k_{1,2}-\mathcal{K}_2\Gamma_2/k_{2,2})}{(k_{1,2}\gamma_{-1,2}+k_{2,2}\gamma_{1,2})^2(\gamma_{1,1}k_{2,2}\mathcal{K}_1+\gamma_{-1,1}k_{1,2}\mathcal{K}_2)} \tag{S.11}$$

with

$$\mathcal{K}_1 = \frac{(1+\gamma_{-1,2}/k_{2,2})k_{1,2} + k_{1,-1} + \gamma_{1,2}}{k^0_{1,1}} \tag{S.12}$$

$$\mathcal{K}_2 = \frac{(1+\gamma_{1,2}/k_{1,2})k_{2,2} + k_{2,-1} + \gamma_{-1,2}}{k^0_{2,1}} \tag{S.13}$$

$$\Gamma_1 = \frac{\gamma_{1,2}}{k_{1,2}} + \frac{\gamma_{-1,2}}{k_{2,2}} + \left(\frac{1}{k_{2,2}} - \frac{1}{k_{1,2}}\right)\gamma_{1,1} \tag{S.14}$$

$$\Gamma_2 = \frac{\gamma_{1,2}}{k_{1,2}} + \frac{\gamma_{-1,2}}{k_{2,2}} + \left(\frac{1}{k_{1,2}} - \frac{1}{k_{2,2}}\right)\gamma_{-1,1} \tag{S.15}$$

Note that $A_0$ and $B_0$ cannot be negative, but $B_1$ can. The conformational current can be written as

$$J_{1,\mathrm{E}} = -\left(\frac{\gamma_{1,2}}{k_{1,2}} + \frac{\gamma_{-1,2}}{k_{2,2}}\right)\frac{f_{1,1}}{[\mathrm{S}] + s_1} \tag{S.16}$$

Also, $\Delta\overline{\Delta\tau^{\mathrm{eff}}}$ can be expressed as

$$\Delta\overline{\Delta\tau^{\mathrm{eff}}} = \frac{\mathcal{K}_1\Gamma_1/k_{1,2} - \mathcal{K}_2\Gamma_2/k_{2,2}}{s_1(\gamma_{1,2}/k_{1,2} + \gamma_{-1,2}/k_{2,2})} \tag{S.17}$$

Thus, we achieve the proportional relationship in eq 7 of the main text.

The reduced parameter $B_1$ vanishes under zero conformational current, which is achieved upon satisfaction of the conformational detailed balance condition

$$\frac{\gamma_{1,1}}{\gamma_{1,2}}K_{1,\mathrm{M}} = \frac{\gamma_{-1,1}}{\gamma_{-1,2}}K_{2,\mathrm{M}} \tag{S.18}$$

Also, $B_1$ can vanish when $\Delta\overline{\Delta\tau^{\mathrm{eff}}} = 0$, which occurs under the following condition:

$$\frac{\mathcal{K}_1\Gamma_1}{k_{1,2}} = \frac{\mathcal{K}_2\Gamma_2}{k_{2,2}} \tag{S.19}$$

This scenario represents a unique type of nonequilibrium symmetry in multidimensional networks. Conformational detailed balance is thus a sufficient but unnecessary condition for MM kinetics. For an analysis of scenarios under which conformational detailed balance is

satisfied, we refer readers to ref 15 of the main text. Lastly, we note that when the constraint mentioned in the main text resulting from local detailed balance, $\gamma_{1,1}k_{1,-1}/(\gamma_{1,2}k^0_{1,1}) = \gamma_{-1,1}k_{2,-1}/(\gamma_{-1,2}k^0_{2,1})$, is obeyed (with nonzero rates), eq S.18 reduces to $k_{1,-1}/k_{1,2} = k_{2,-1}/k_{2,2}$, which is satisfied when the ratio of the unbinding and catalytic rates is conformation invariant.
